# Supplementary material for: A Matsuoka-Based GARMA Model for Hydrological Forecasting: Theory, Estimation, and Applications
Source: arXiv:2502.18645 source file (2025-02-25)
Supplement: Supplementary file 1 [file sup_mat.pdf]

# A Matsuoka-Based GARMA Model for Hydrological Forecasting: Theory, Estimation, and Applications

## Supplementary Material

Guilherme Pumi<sup>a,\*</sup>, Danilo Hiroshi Matsuoka<sup>a</sup>, Taiane Schaedler Prass<sup>a</sup> and  
Bruna G. Palm<sup>b</sup>

### Introduction

Due to page restrictions, in this document we present some plots excluded from the parent paper. We reproduce parts of the paper to contextualize the simulation, Please refer to the parent paper for more details regarding the results presented here.

We generate samples of size  $n \in \{100, 200, 500\}$  from an MARMA(1, 1) model with parameters  $\alpha \in \{0.5, 1\}$ ,  $(\phi, \theta) \in \{(0.2, -0.8), (-0.8, 0.2), (-0.4, -0.2), (0.4, 0.2)\}$ , considering a sinusoidal covariate given by  $x_t = \sin(\pi t/50)$  with coefficient  $\beta = -0.5$ . A size 100 burn-in is applied in generating the time series. We consider the cloglog link function in our experiments. A total of 1,000 replicas of each scenario were generated. Routines to sample from an MARMA( $p, q$ ) process and to perform estimation via PMLE are available in R package BTSR (Prass and Pumi, 2022).

Below we examine pairwise scatter plots and marginal behavior (histograms and boxplots). From the scatter plots, we observe the convergence of the points to a familiar Gaussian behavior as  $n$  increases. The marginal behavior (histograms and boxplots) overall becomes more symmetrical as  $n$  increases, with the histograms resembling the shape of a normal distribution. It is also noteworthy that there is dependence between the estimates of parameters  $\alpha$ ,  $\phi$ , and  $\theta$ , whose pairwise plots are located in the right column of each figure. In sharp contrast, the estimates of  $\beta$  are uncorrelated with the other parameters, as seen in the plots in the left column of each Figure.

---

\*Corresponding author. This Version: February 25, 2025

<sup>a</sup>Mathematics and Statistics Institute and Programa de Pós-Graduação em Estatística - Universidade Federal do Rio Grande do Sul, Brazil.

<sup>b</sup>Department of Mathematics and Natural Sciences - Blekinge Institute of Technology, Sweden.

E-mails: guilherme.pumi@ufrgs.br (Pumi), danilomatsuoka@gmail.com (Matsuoka), taiane.prass@ufrgs.br (Prass), bruna.palm@bth.se (Palm)

ORCID: 0000-0002-6256-3170 (Pumi); 0000-0002-9744-8260 (Matsuoka); 0000-0003-3136-909X (Prass); 0000-0003-0423-9927 (Palm).

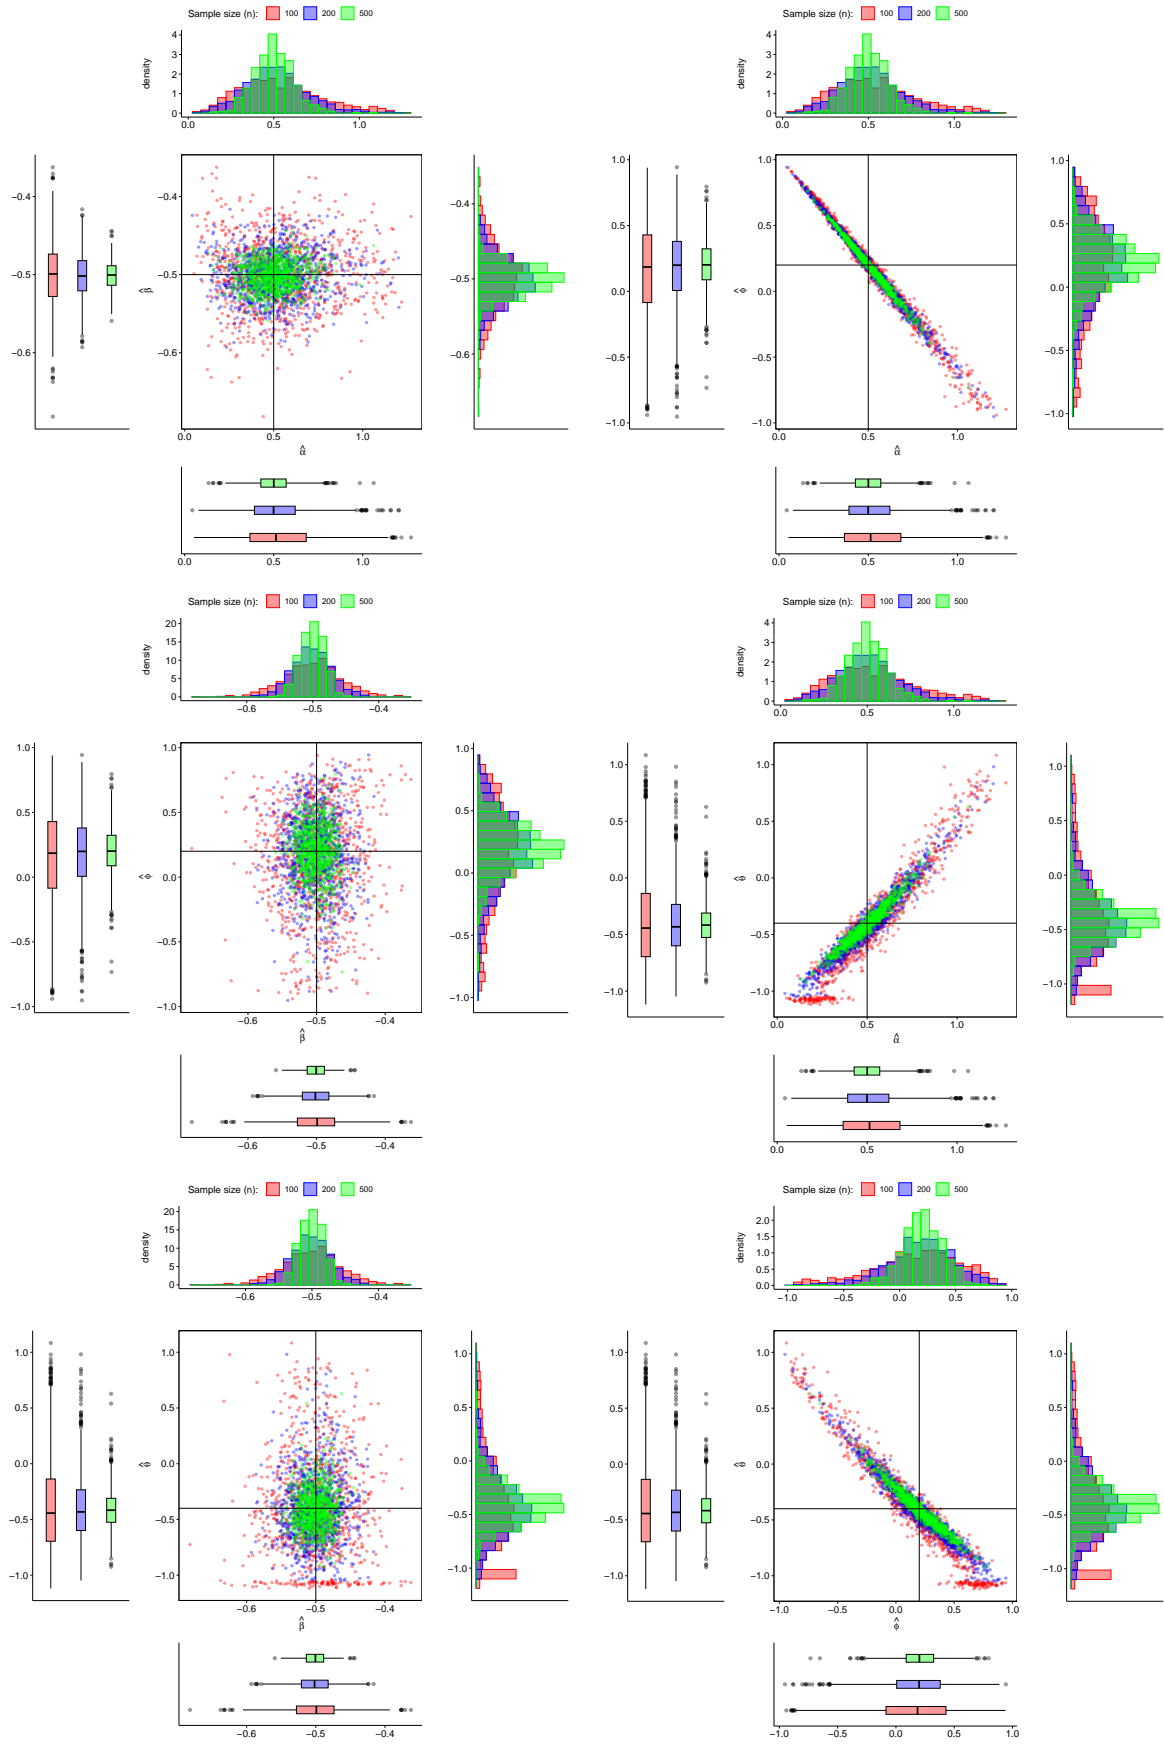

Figure 1: Pairwise joint and marginal behavior of the estimated values for  $\alpha = 0.5$ ,  $\beta = -0.5$ ,  $\phi = 0.2$ ,  $\theta = -0.4$ .

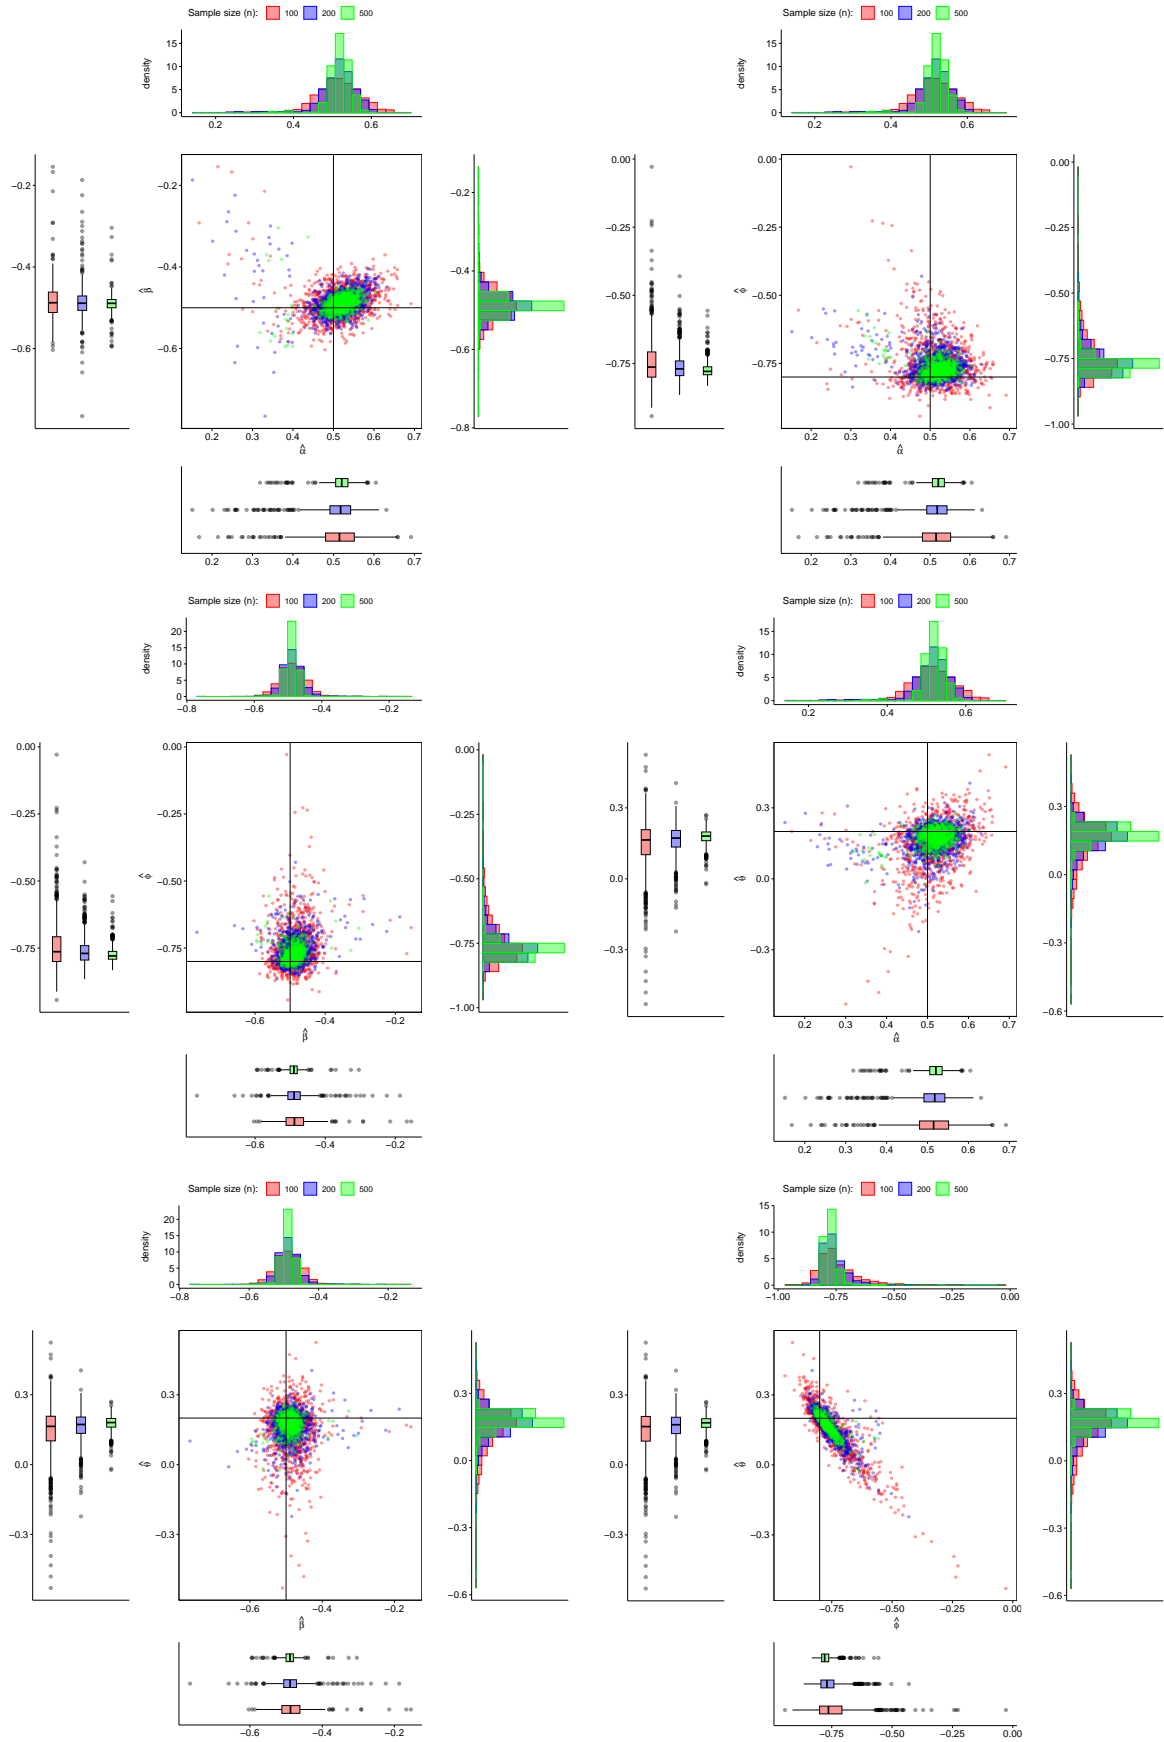

Figure 2: Pairwise joint and marginal behavior of the estimated values for  $\alpha = 0.5$ ,  $\beta = -0.5$ ,  $\phi = -0.8$ ,  $\theta = 0.2$ .

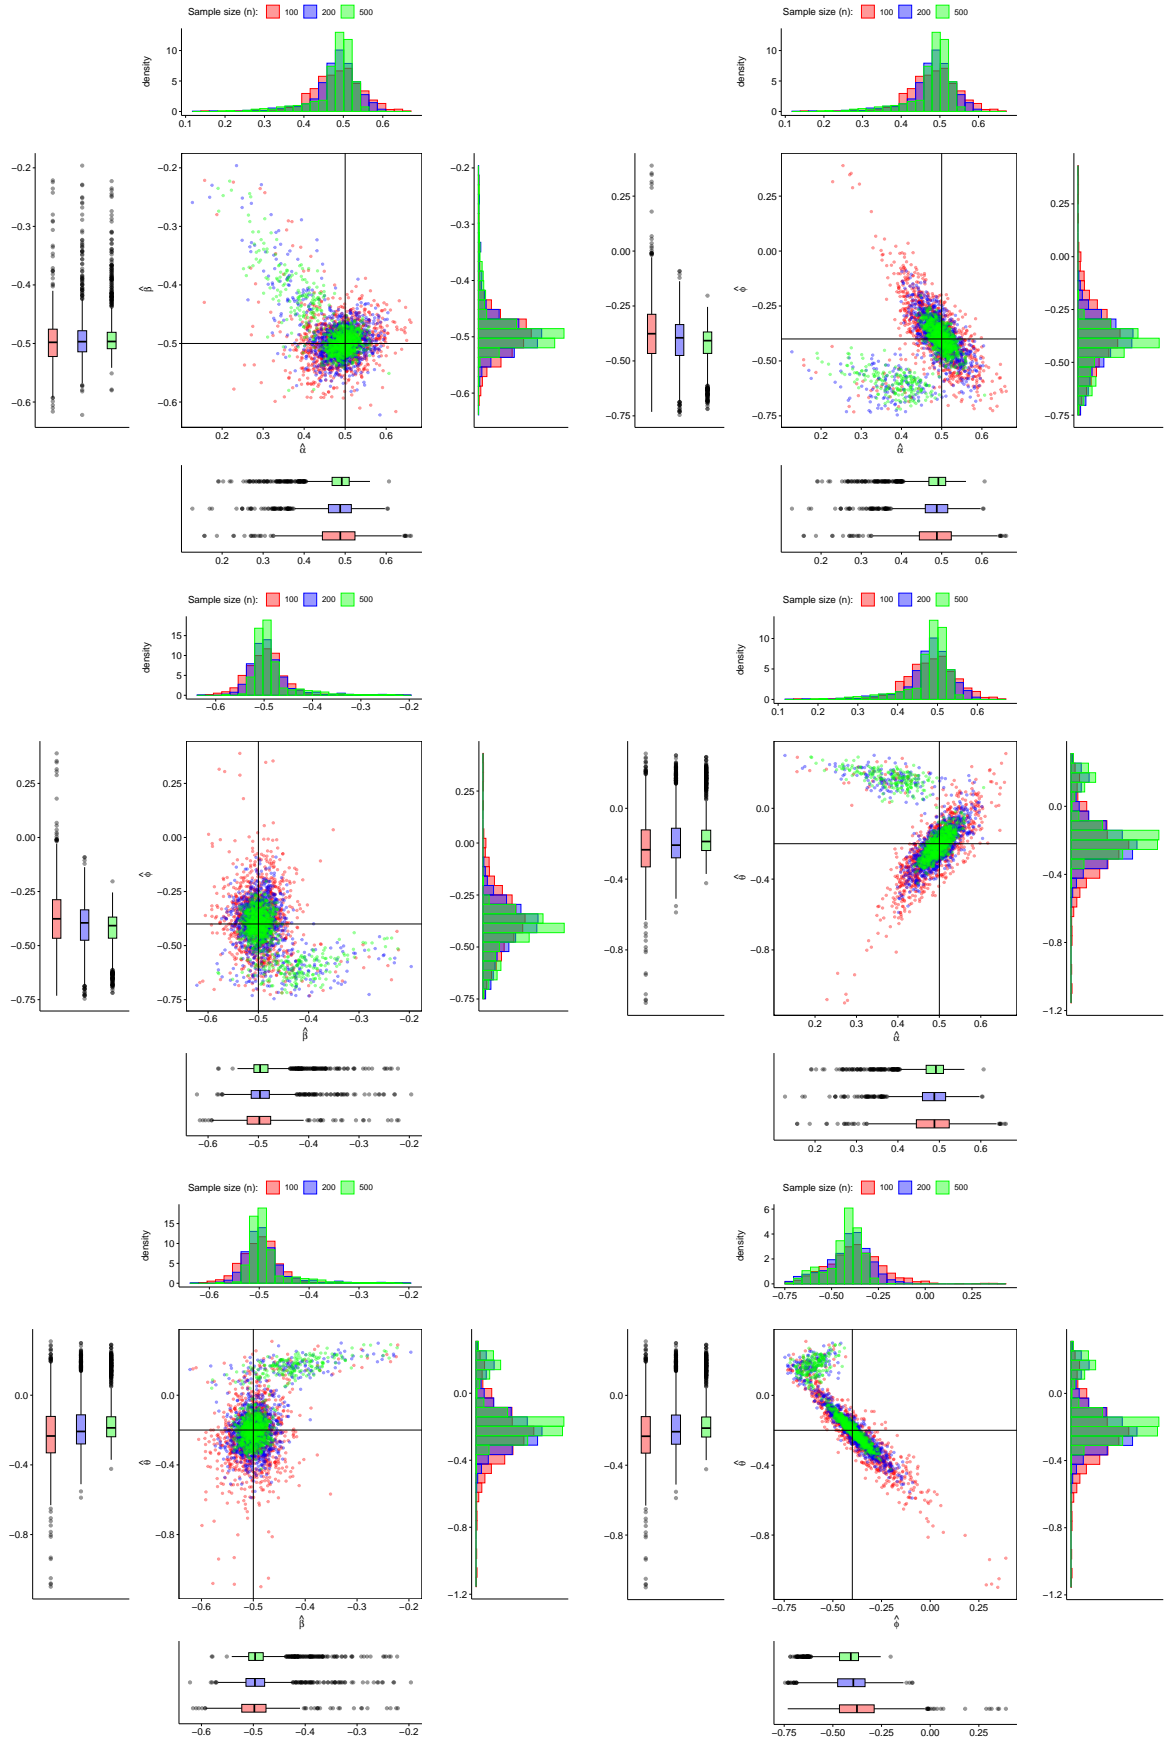

Figure 3: Pairwise joint and marginal behavior of the estimated values for  $\alpha = 0.5$ ,  $\beta = -0.5$ ,  $\phi = -0.4$ ,  $\theta = -0.2$ .



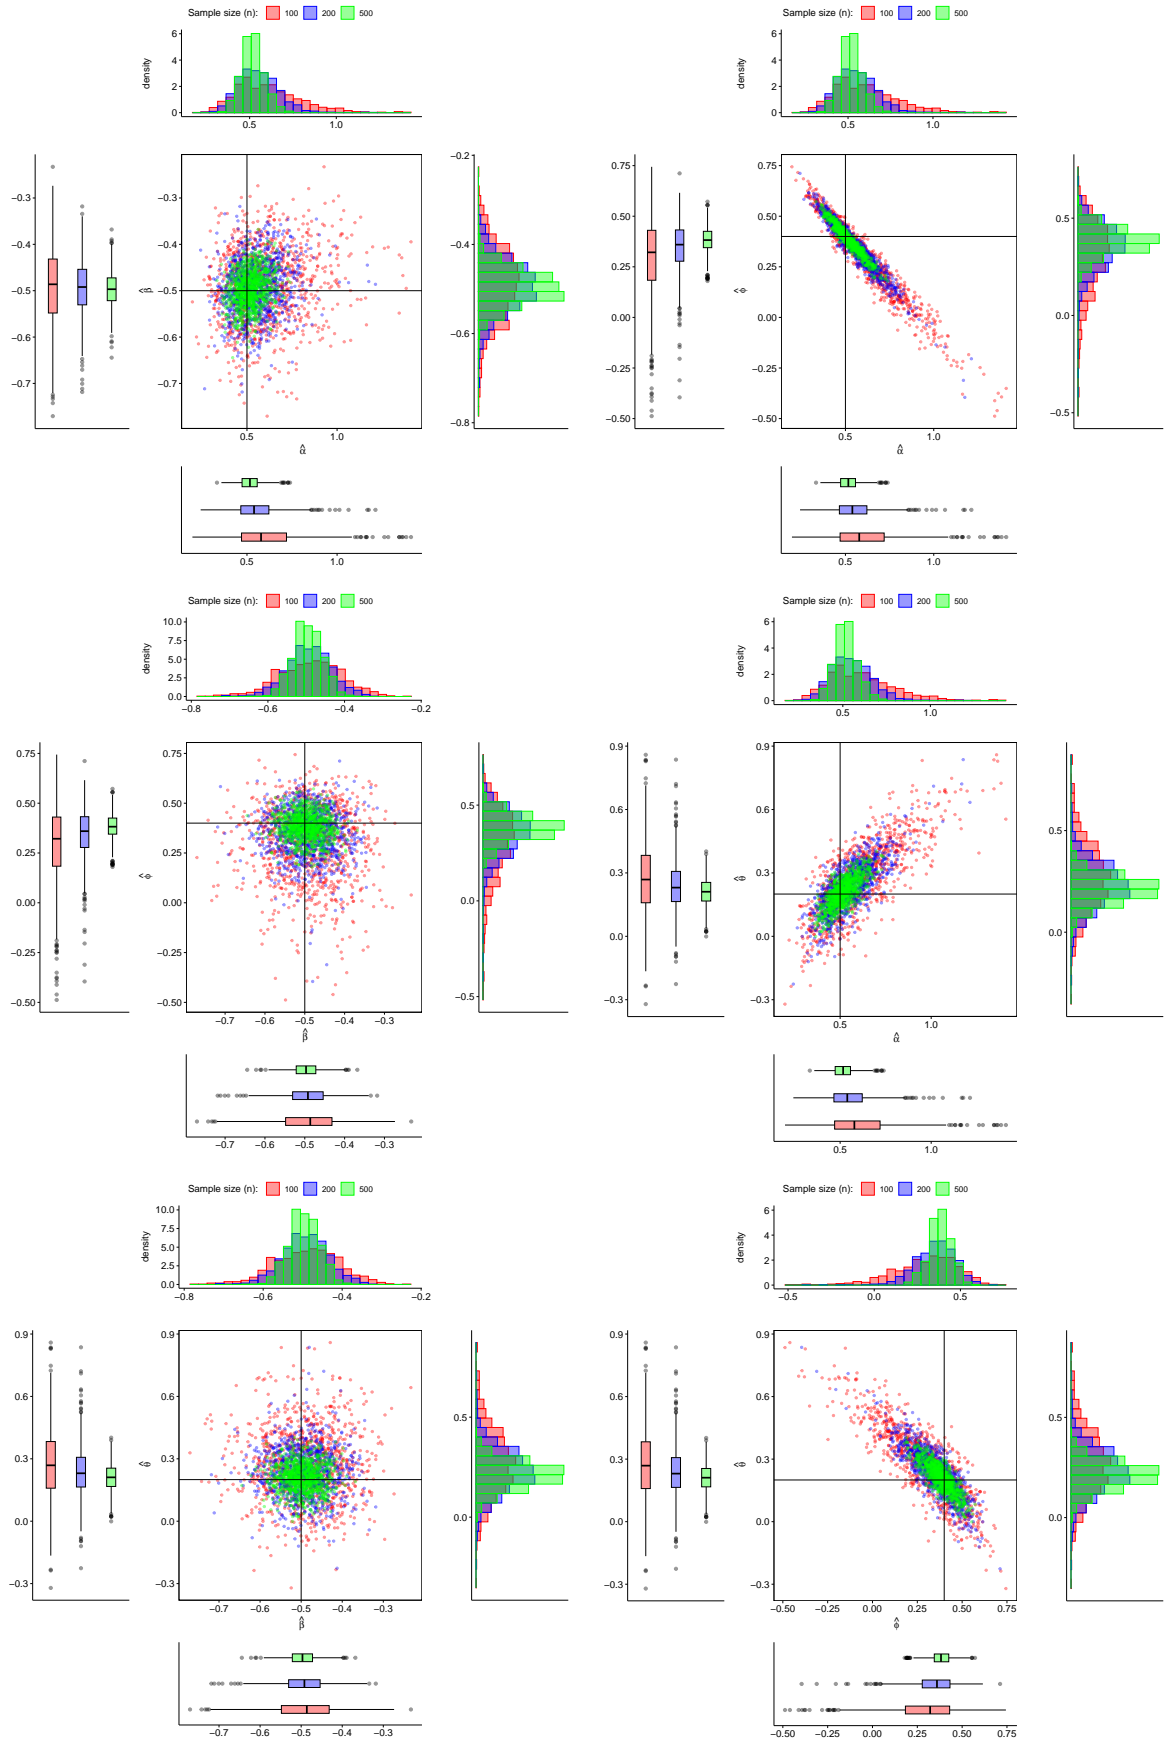

Figure 4: Pairwise joint and marginal behavior of the estimated values for  $\alpha = 0.5$ ,  $\beta = -0.5$ ,  $\phi = 0.4$ ,  $\theta = 0.2$ .

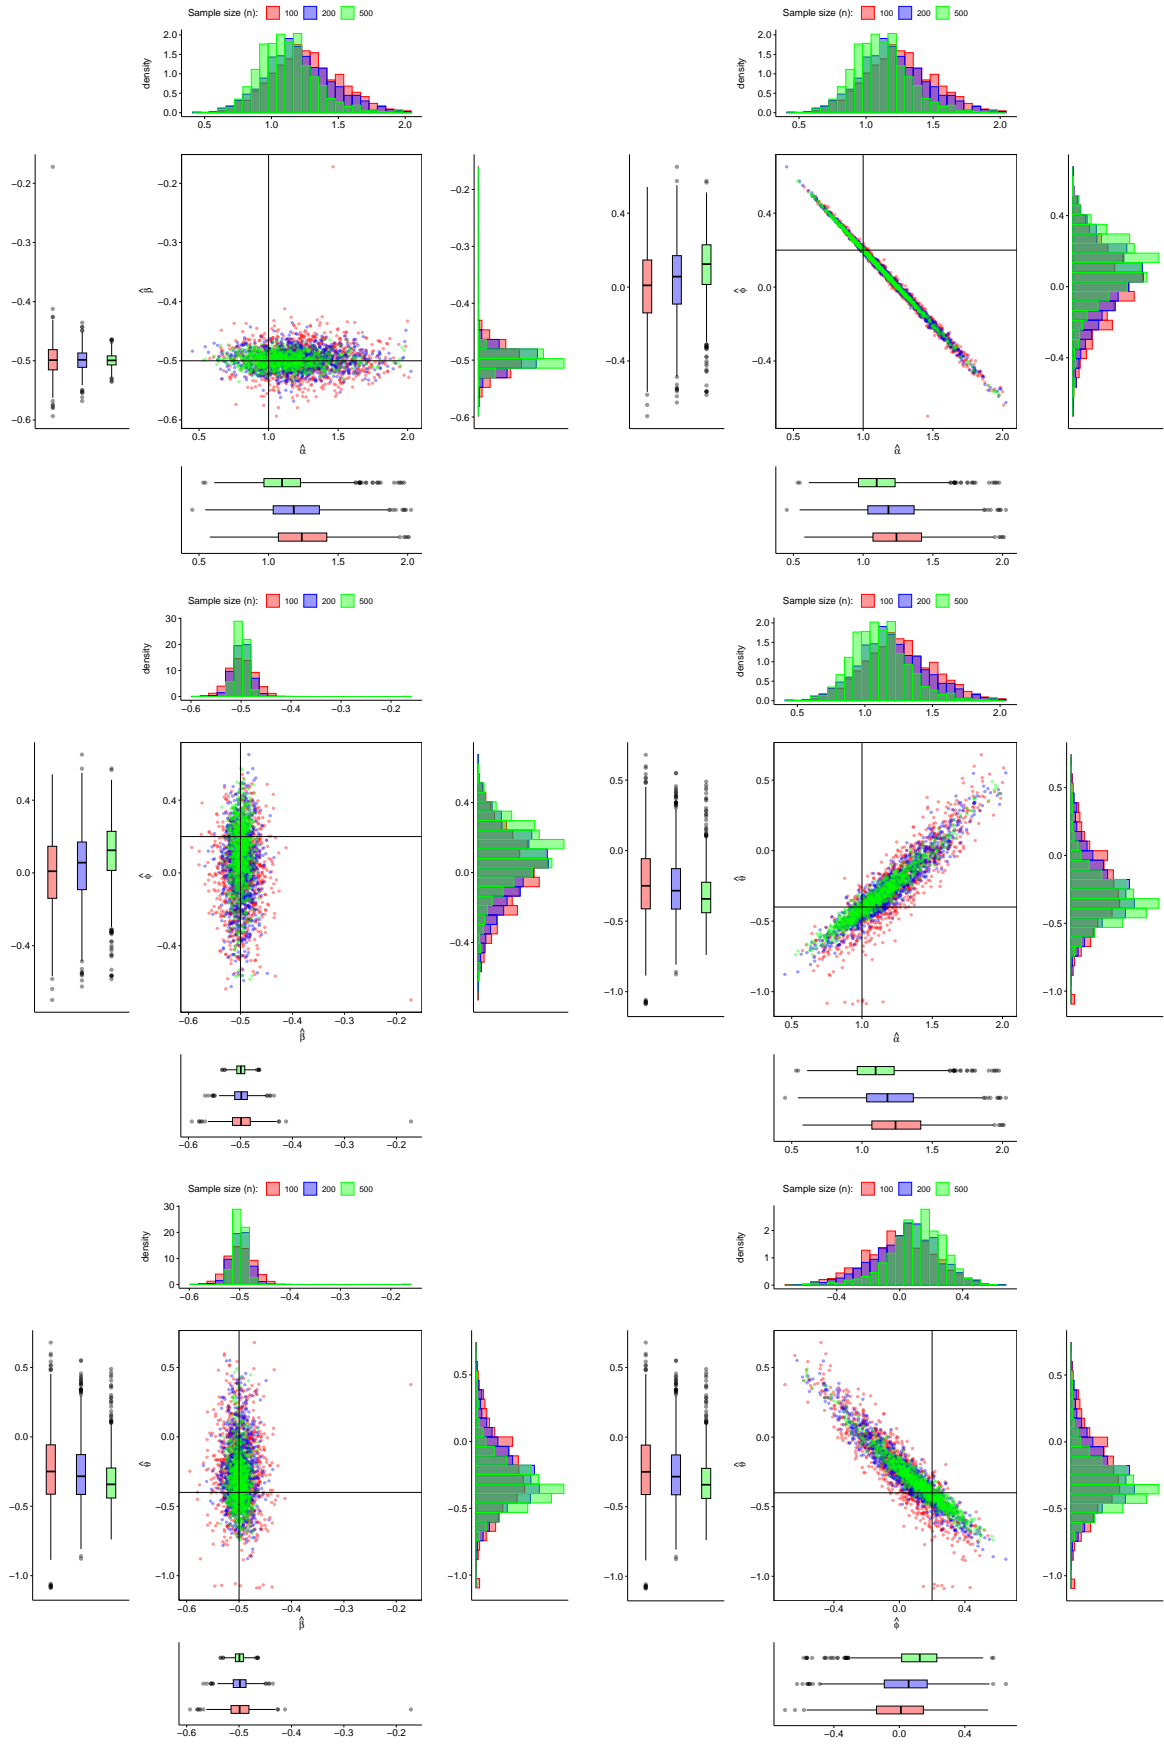

Figure 5: Pairwise joint and marginal behavior of the estimated values for  $\alpha = 1$ ,  $\beta = -0.5$ ,  $\phi = -0.2$ ,  $\theta = 0.4$ .

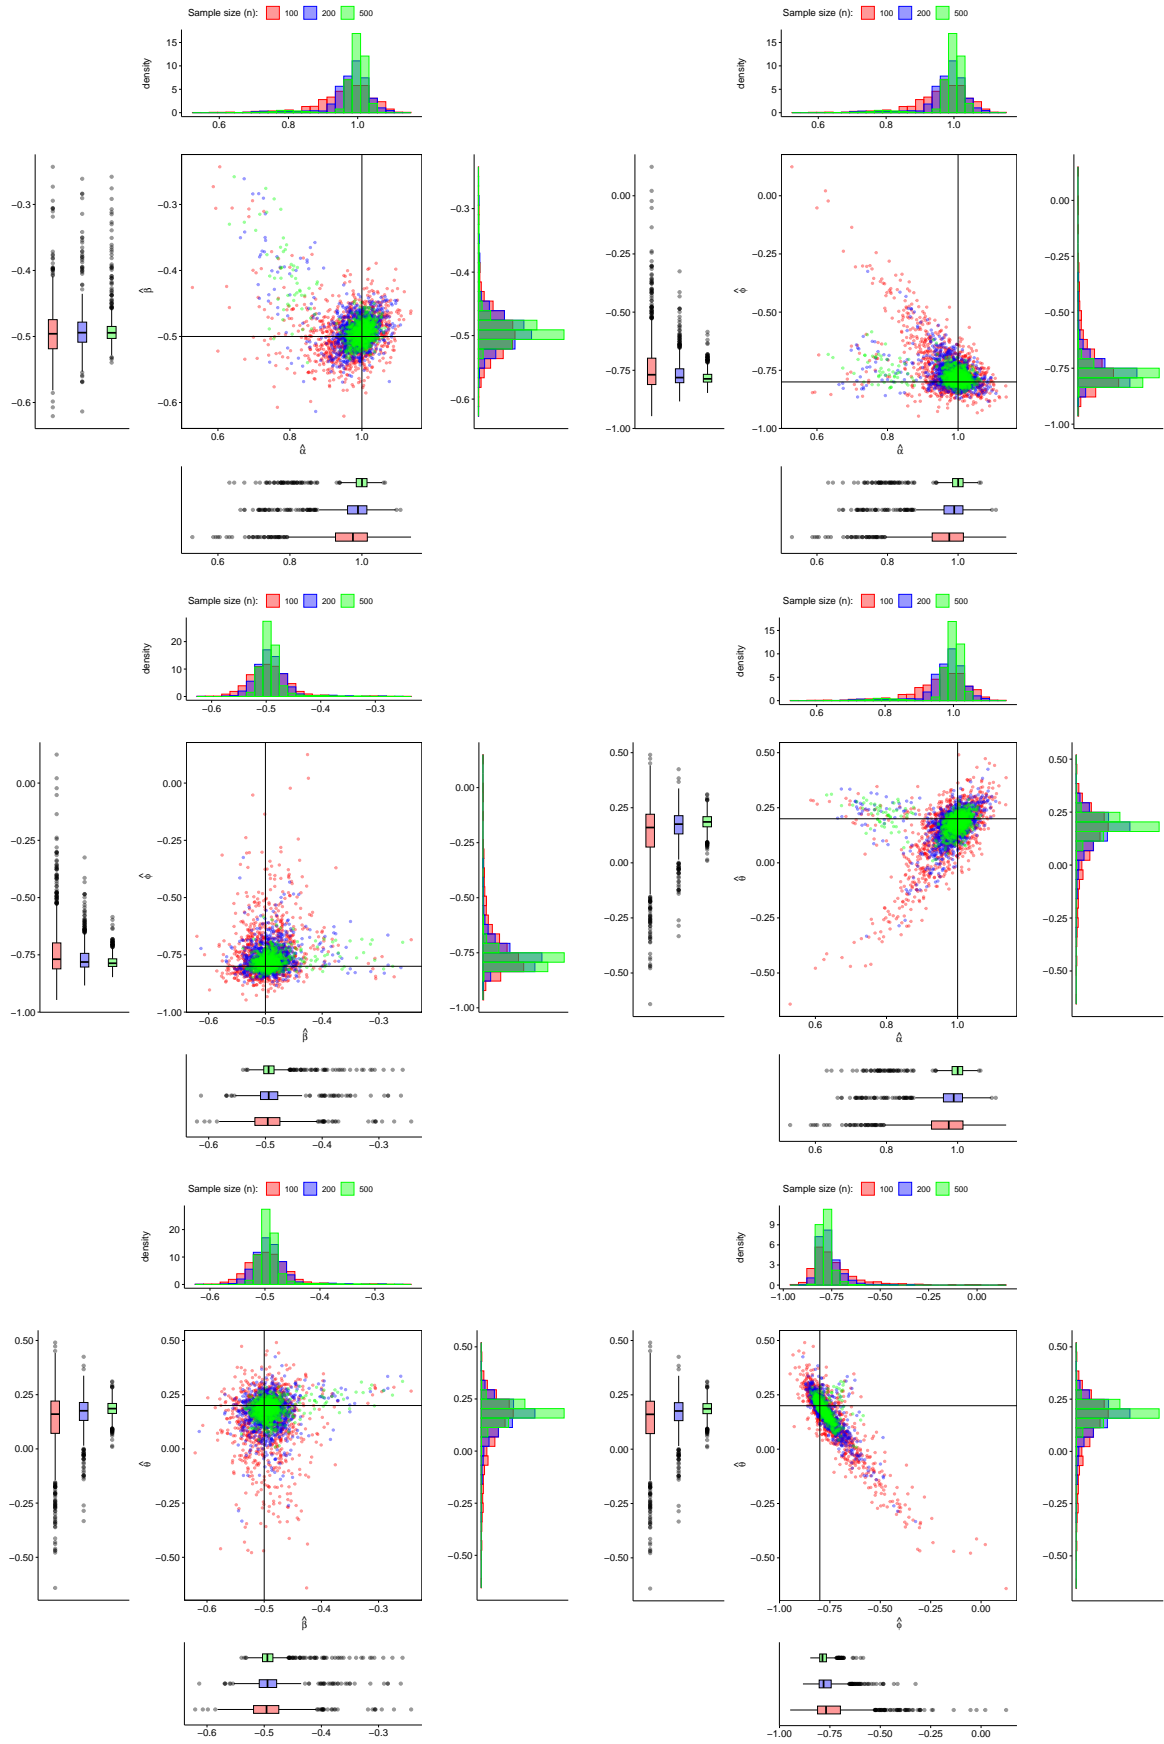

Figure 6: Pairwise joint and marginal behavior of the estimated values for  $\alpha = 1$ ,  $\beta = -0.5$ ,  $\phi = -0.8$ ,  $\theta = 0.2$ .

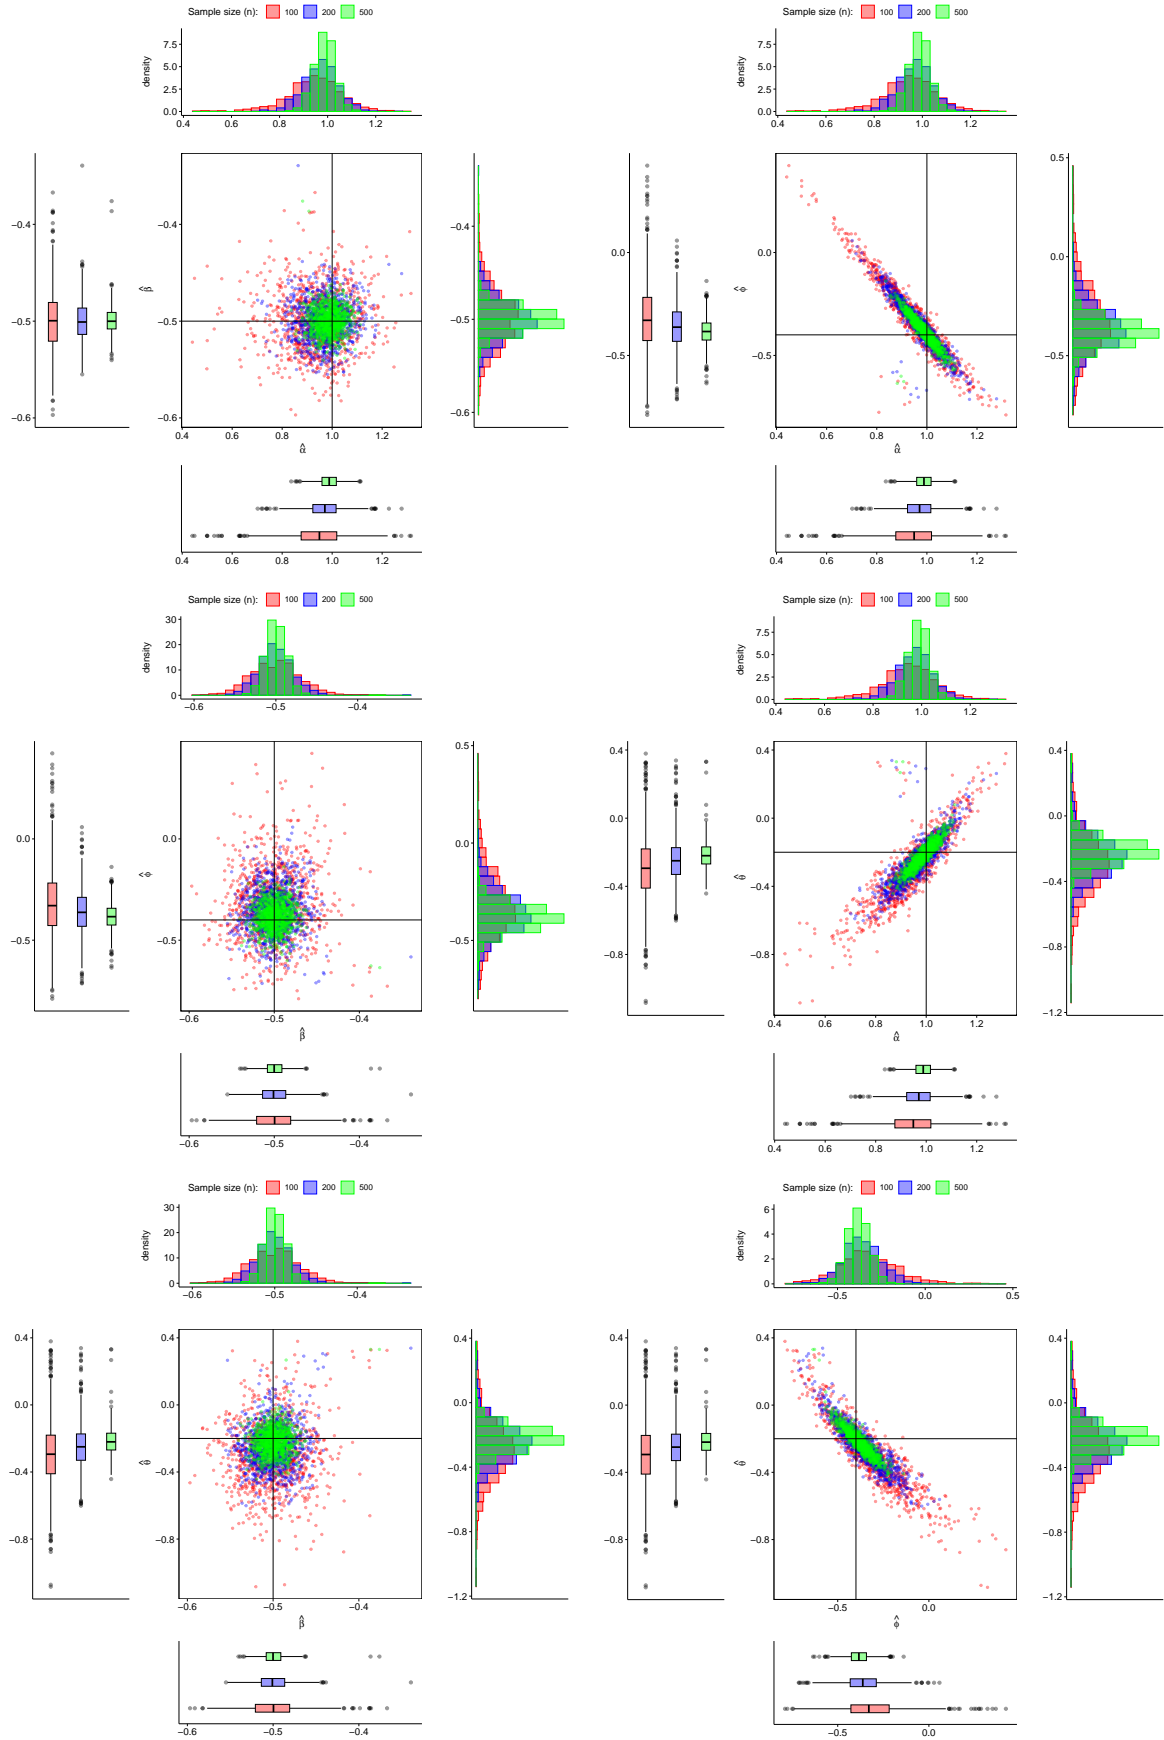

Figure 7: Pairwise joint and marginal behavior of the estimated values for  $\alpha = 1$ ,  $\beta = -0.5$ ,  $\phi = -0.4$ ,  $\theta = -0.2$ .

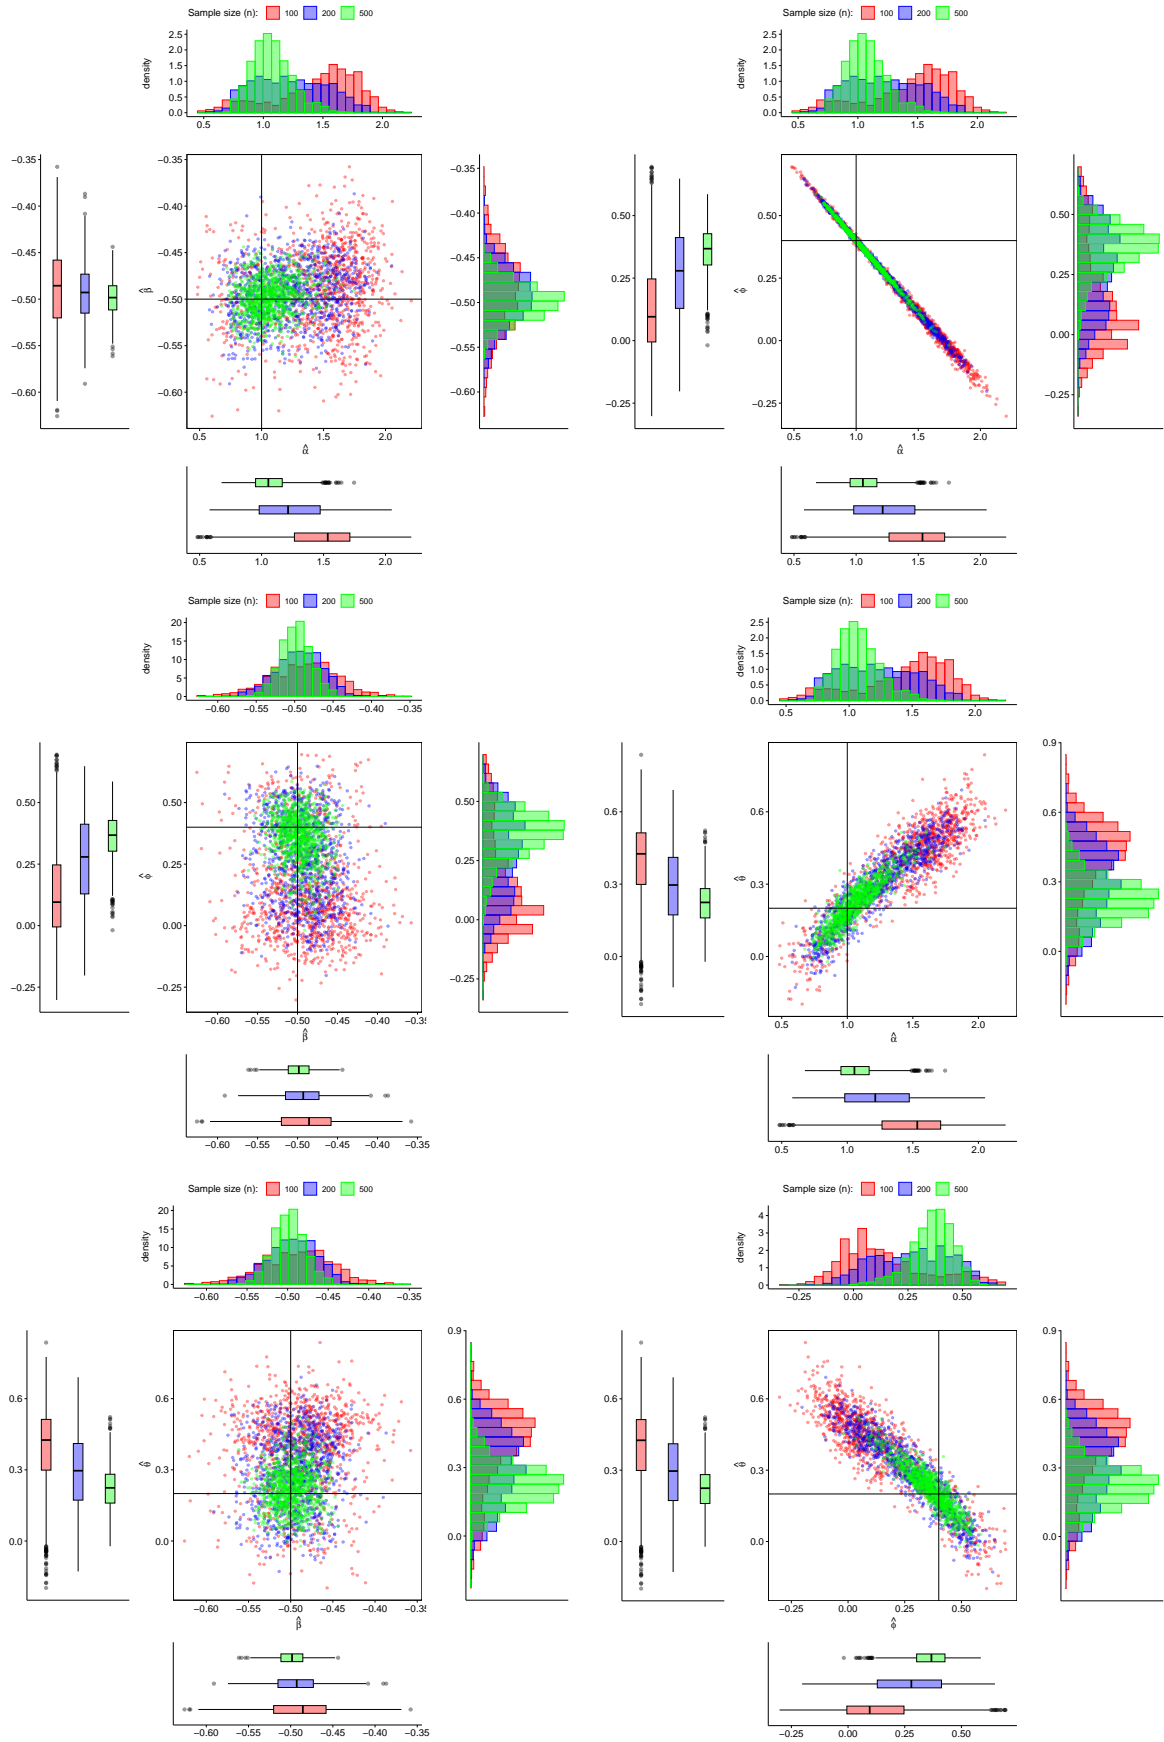

Figure 8: Pairwise joint and marginal behavior of the estimated values for  $\alpha = 1$ ,  $\beta = -0.5$ ,  $\phi = 0.4$ ,  $\theta = 0.2$ .

## References

`btsr`

Prass, T. S. and Pumi, G. (2022). *BTSR: Bounded Time Series Regression*. R package version 0.1.0.
